# Supplementary material for: Unambiguous fluctuation decomposition of the self-energy: pseudogap physics beyond spin fluctuations
Source: arXiv:2401.08543 ancillary file (2024-05-26)
Supplement: Supplementary file 1 [file supplement.pdf]

# Supplemental Material:
# Unambiguous fluctuation decomposition of the self-energy: pseudogap physics beyond spin fluctuations

Yang Yu,[1] Sergei Iskakov,[1] Emanuel Gull,[1] Karsten Held,[2] and Friedrich Krien[2]

[1] *Department of Physics, University of Michigan, Ann Arbor, MI 48109, USA*

[2] *Institute for Solid State Physics, TU Wien, 1040 Vienna, Austria*

In this supplementary material, we elaborate on the fluctuation decomposition introduced in the main text, along with additional computational findings mentioned in the main text. Section I details the definitions of various quantities involved in the fluctuation decomposition. Section II delves into the derivation of the fluctuation decomposition, demonstrating the uniqueness of the formalism. Furthermore, Sec. III provides supplementary results from DMFT (dynamical mean-field theory) and DCA (dynamical cluster approximation) calculations, which include results in different parameter regimes, high-frequency tails of the different terms in the fluctuation decomposition, and the decomposition of the multi-boson term.

## I. SINGLE-BOSON EXCHANGE QUANTITIES

In this section, we provide definitions for the quantities used in the fluctuation decomposition. These include the susceptibilities $\chi_q$, the Hedin vertices $\gamma_{kq}$, and the screened interactions $W_q$. In our definitions we follow mostly Ref. [1], except for a factor $\frac{1}{2}$ for the susceptibilities $\chi^{\mathrm{ch/sp}}$ (see below), and wiggly lines in Fig. 1 of the main manuscript denote $\chi$ rather than the screened interaction $W$. As in the main text, summation over a momentum-frequency vector $k$ or $q$ implies multiplication with a factor $\frac{T}{N}$. Additionally, in the following derivation, we implicitly assume SU(2) symmetry for the spin degree of freedom.

For practical applications, we employ the dynamical cluster approximation (DCA) along with a continuous-time quantum Monte Carlo method as the impurity solver [2–5]. In the following discussion, the momentum in the calculation results specifically represents the cluster momentum. However, it should be noted that, beyond the DCA, the formulas below are equally applicable to the lattice momentum.

DCA is used to calculate the one-body Green's function $G_{k\sigma} = -\langle \hat{c}_{k\sigma}\hat{c}^\dagger_{k\sigma}\rangle$ and the two-body Green's functions $G^{(2),\mathrm{ph/pp}}_{kk'q,\sigma\sigma'}$:

$$G^{(2),\mathrm{ph}}_{kk'q,\uparrow\uparrow} = -\left\langle \hat{c}_{k\uparrow}\hat{c}^\dagger_{(k+q)\uparrow}\hat{c}_{(k'+q)\uparrow}\hat{c}^\dagger_{k'\uparrow}\right\rangle, \tag{S1a}$$

$$G^{(2),\mathrm{ph}}_{kk'q,\uparrow\downarrow} = -\left\langle \hat{c}_{k\uparrow}\hat{c}^\dagger_{(k+q)\uparrow}\hat{c}_{(k'+q)\downarrow}\hat{c}^\dagger_{k'\downarrow}\right\rangle, \tag{S1b}$$

$$G^{(2),\mathrm{pp}}_{kk'q,\uparrow\uparrow} = \left\langle \hat{c}_{k\uparrow}\hat{c}_{(q-k)\uparrow}\hat{c}^\dagger_{(q-k')\uparrow}\hat{c}^\dagger_{k'\uparrow}\right\rangle, \tag{S1c}$$

$$G^{(2),\mathrm{pp}}_{kk'q,\uparrow\downarrow} = \left\langle \hat{c}_{k\uparrow}\hat{c}_{(q-k)\downarrow}\hat{c}^\dagger_{(q-k')\uparrow}\hat{c}^\dagger_{k'\downarrow}\right\rangle. \tag{S1d}$$

where ph (pp) denotes the particle-hole (particle-particle) channel. The generalized susceptibilities $\chi^{\mathrm{ph/pp}}_{kk'q,\sigma\sigma'}$ are obtained via removing the direct contribution $\sim G_kG_{k'}$:

$$\chi^{\mathrm{ph}}_{kk'q,\uparrow\uparrow} = G^{(2),\mathrm{ph}}_{kk'q,\uparrow\uparrow} + \frac{N}{T}G_{k\uparrow}G_{k'\uparrow}\delta_q, \tag{S2a}$$

$$\chi^{\mathrm{ph}}_{kk'q,\uparrow\downarrow} = G^{(2),\mathrm{ph}}_{kk'q,\uparrow\downarrow} + \frac{N}{T}G_{k\uparrow}G_{k'\downarrow}\delta_q, \tag{S2b}$$

$$\chi^{\mathrm{pp}}_{kk'q,\uparrow\uparrow} = G^{(2),\mathrm{pp}}_{kk'q,\uparrow\uparrow} + \frac{N}{T}G_{k\uparrow}G_{k'\uparrow}\delta_{q-k-k'}, \tag{S2c}$$

$$\chi^{\mathrm{pp}}_{kk'q,\uparrow\downarrow} = G^{(2),\mathrm{pp}}_{kk'q,\uparrow\downarrow} + \frac{N}{T}G_{k\uparrow}G_{k'\downarrow}\delta_{q-k-k'}. \tag{S2d}$$

The generalized susceptibilities in the charge/spin/singlet (abbreviated as ch/sp/si) channels are defined as

$$\chi^{\text{ch}}_{kk'q} = \chi^{\text{ph}}_{kk'q,\uparrow\uparrow} + \chi^{\text{ph}}_{kk'q,\uparrow\downarrow}, \tag{S3a}$$
$$\chi^{\text{sp}}_{kk'q} = \chi^{\text{ph}}_{kk'q,\uparrow\uparrow} - \chi^{\text{ph}}_{kk'q,\uparrow\downarrow}, \tag{S3b}$$
$$\chi^{\text{si}}_{kk'q} = \frac{1}{2}\left(-\chi^{\text{pp}}_{kk'q,\uparrow\uparrow} + 2\chi^{\text{pp}}_{kk'q,\uparrow\downarrow} - \frac{N}{T}G_{k\uparrow}G_{(q-k)\downarrow}\delta_{k-k'}\right). \tag{S3c}$$

The physical susceptibilities $\chi_q^{\text{ch/sp/si}}$ are then obtained via summing over $k'$ and $k$:

$$\chi_q^{\text{ch/sp/si}} = \sum_{kk'} \chi^{\text{ch/sp/si}}_{kk'q}. \tag{S4}$$

Based on the above definition one can show that ($qx \equiv \mathbf{q}\cdot\mathbf{x} + \omega\tau$)

$$\chi^{\text{ch}}_q = -\frac{1}{2}\sum_x \mathrm{e}^{-\mathrm{i}qx}[\langle \mathcal{T}_\tau \hat{n}_x \hat{n}_0\rangle - \langle \hat{n}_0\rangle^2], \tag{S5a}$$
$$\chi^{\text{sp}}_q = -\frac{1}{2}\sum_x \mathrm{e}^{-\mathrm{i}qx}\left\langle \mathcal{T}_\tau \hat{m}_x \hat{m}_0\right\rangle, \tag{S5b}$$
$$\chi^{\text{si}}_q = -\sum_x \mathrm{e}^{\mathrm{i}qx}\left\langle \mathcal{T}_\tau \hat{\rho}^-_x \hat{\rho}^+_0\right\rangle, \tag{S5c}$$

where $\hat{\rho}^-_x = \hat{c}_{x\downarrow}\hat{c}_{x\uparrow}$, $\hat{\rho}^+_x = \hat{c}^\dagger_{x\uparrow}\hat{c}^\dagger_{x\downarrow}$, $\hat{n}_x = \hat{c}^\dagger_{x\uparrow}\hat{c}_{x\uparrow} + \hat{c}^\dagger_{x\downarrow}\hat{c}_{x\downarrow}$ and $\hat{m}_x = \hat{c}^\dagger_{x\uparrow}\hat{c}_{x\uparrow} - \hat{c}^\dagger_{x\downarrow}\hat{c}_{x\downarrow}$. (Notice that our definition of $\chi^{\text{ch/sp}}$ differs by a factor of $\frac{1}{2}$ from Ref. [6].) The screened interactions $W_q^{\text{ch/sp/si}}$ are defined as

$$W^{\text{ch}}_q = U^{\text{ch}} + U^{\text{ch}}\chi^{\text{ch}}_q U^{\text{ch}} = U + U^2\chi^{\text{ch}}_q, \tag{S6a}$$
$$W^{\text{sp}}_q = U^{\text{sp}} + U^{\text{sp}}\chi^{\text{sp}}_q U^{\text{sp}} = -U + U^2\chi^{\text{sp}}_q, \tag{S6b}$$
$$W^{\text{si}}_q = U^{\text{si}} + \frac{1}{2}U^{\text{si}}\chi^{\text{si}}_q U^{\text{si}} = 2U + 2U^2\chi^{\text{si}}_q, \tag{S6c}$$

where $U^{\text{ch}} = U$, $U^{\text{sp}} = -U$, and $U^{\text{si}} = 2U$.

The vertex functions $F^{\text{ch/sp/si}}_{kk'q}$ can be obtained from the relations ($G_k \equiv G_{k\uparrow} = G_{k\downarrow}$ here and below)

$$\chi^{\text{ch/sp}}_{kk'q} = \frac{N}{T}\delta_{k-k'}G_kG_{k+q} + G_kG_{k+q}F^{\text{ch/sp}}_{kk'q}G_{k'}G_{k'+q}, \tag{S7a}$$
$$\chi^{\text{si}}_{kk'q} = -\frac{N}{T}\delta_{k-k'}G_kG_{q-k} + \frac{1}{2}G_kG_{q-k}F^{\text{si}}_{kk'q}G_{k'}G_{q-k'}. \tag{S7b}$$

The Hedin vertices $\gamma^{\text{ch/sp/si}}_{kq}$ are obtained via

$$\gamma^{\text{ch}}_{kq} = \frac{1 + \sum_{k'} F^{\text{ch}}_{kk'q}G_{k'}G_{k'+q}}{1 + U\chi^{\text{ch/sp}}_q}, \tag{S8a}$$
$$\gamma^{\text{sp}}_{kq} = \frac{1 + \sum_{k'} F^{\text{sp}}_{kk'q}G_{k'}G_{k'+q}}{1 - U\chi^{\text{sp}}_q}, \tag{S8b}$$
$$\gamma^{\text{si}}_{kq} = \frac{-1 + \frac{1}{2}\sum_{k'} F^{\text{si}}_{kk'q}G_{k'}G_{q-k'}}{1 + U\chi^{\text{si}}_q}. \tag{S8c}$$

## II. FLUCTUATION DECOMPOSITION

Ref. [7] introduced the fluctuation diagnostics of the self-energy, which may be compactly written as follows,

$$\Sigma_k - \Sigma^H = -U\sum_{k'q} G_{k+q}G_{k'}G_{k'+q}\left[rF^{\text{ch}}_{kk'q} + (r-1)F^{\text{sp}}_{kk'q}\right], \tag{S9}$$

where $r=1$, $r=0$, and $r=\frac{1}{4}$ lead to the charge, spin, or particle-particle picture, respectively. In the latter case the connection to the singlet particle-particle vertex function is made through $F^{\rm si}_{kk'q}=\frac{1}{2}(F^{\rm ch}_{kk',q-k-k'}-3F^{\rm sp}_{kk',q-k-k'})$ and the sum over the bosonic index is shifted: $q\to q-k-k'$.

Notice that the sums in Eq. (S9) converge in general only if a convergence factor is added, whereas for $r=\frac{1}{2}$ a convergence factor is not needed. Also, Eq. (S9) can be derived for any real number $0\le r\le 1$ due to the relation for the Hubbard interaction, $U\hat{n}_\uparrow\hat{n}_\downarrow = U\frac{r\hat{n}\hat{n}+(r-1)\hat{m}\hat{m}}{2}-(r-\frac{1}{2})U\hat{n}$, where the lattice site index has been dropped. In practice one needs to take a shift of the chemical potential into account that arises for $r\neq\frac{1}{2}$.

The equivalence of the fluctuation decomposition used in the main text with all three pictures introduced in Ref. [7] is shown by partially eliminating the parameter $r$ as follows. We recall the single-boson exchange (SBE) decomposition introduced in Ref. [6],

$$F^{\alpha={\rm ch/sp}}_{kk'q}=\Delta^{{\rm ph},\alpha}_{kk'q}+\Delta^{\overline{\rm ph},\alpha}_{kk'q}+\Delta^{{\rm pp},\alpha}_{kk',k+k'+q}+\Lambda^{{\rm Uirr},\alpha}_{kk'q}-2U^\alpha. \tag{S10}$$

Here $\Delta$ and $\Lambda^{\rm Uirr}$ denote single- and multi-boson exchange, respectively. The SBE vertices are given as (see Eqs. (10), (13), and (20) of Ref. [6]),

$$\Delta^{{\rm ph},\alpha}_{kk'q}=\gamma^\alpha_{kq}W^\alpha_q\gamma^\alpha_{k'q} \tag{S11a}$$
$$\Delta^{\overline{\rm ph},\alpha}_{kk'q}=-\frac{1}{2}\Delta^{\rm ph,ch}_{k,k+q,k'-k}-\frac{3-4\delta_{\alpha,{\rm sp}}}{2}\Delta^{\rm ph,sp}_{k,k+q,k'-k}, \tag{S11b}$$
$$\Delta^{{\rm pp},\alpha}_{kk'q}=\frac{1-2\delta_{\alpha,{\rm sp}}}{2}\gamma^{\rm si}_{kq}W^{\rm si}_q\gamma^{\rm si}_{k'q}\equiv\frac{1-2\delta_{\alpha,{\rm sp}}}{2}\Delta^{\rm pp,si}_{kk'q}, \tag{S11c}$$

where $\gamma$ and $W$ denote the Hedin three-leg vertex and the screened interaction of the indicated flavor, as defined in Eqs. (S6) and (S8). Inserting the SBE decomposition (S10) into Eq. (S9) we obtain

$$\begin{aligned}\Sigma_k-\Sigma^H=&-U\sum_{k'q}G_{k+q}G_{k'}G_{k'+q}\left[r\Delta^{\rm ph,ch}_{kk'q}+(r-1)\Delta^{\rm ph,sp}_{kk'q}\right]\\&-U\sum_{k'q}G_{k+q}G_{k'}G_{k'+q}\left[r\Delta^{\overline{\rm ph},{\rm ch}}_{kk'q}+(r-1)\Delta^{\overline{\rm ph},{\rm sp}}_{kk'q}\right]\\&-U\sum_{k'q}G_{k+q}G_{k'}G_{k'+q}\left[r\Delta^{\rm pp,ch}_{kk',k+k'+q}+(r-1)\Delta^{\rm pp,sp}_{kk',k+k'+q}\right]\\&-U\sum_{k'q}G_{k+q}G_{k'}G_{k'+q}\left[r\Lambda^{\rm Uirr,ch}_{kk'q}+(r-1)\Lambda^{\rm Uirr,sp}_{kk'q}\right]\\&+2U\sum_{k'q}G_{k+q}G_{k'}G_{k'+q}\left[rU^{\rm ch}+(r-1)U^{\rm sp}\right].\end{aligned} \tag{S12}$$

Similarly, inserting Eq. (S11b) into the expression inside the square bracket in the second line, we obtain

$$\begin{aligned}&r\Delta^{\overline{\rm ph},{\rm ch}}_{kk'q}+(r-1)\Delta^{\overline{\rm ph},{\rm sp}}_{kk'q}\\&=r\left(-\frac{1}{2}\Delta^{\rm ph,ch}_{k,k+q,k'-k}-\frac{3}{2}\Delta^{\rm ph,sp}_{k,k+q,k'-k}\right)+(r-1)\left(-\frac{1}{2}\Delta^{\rm ph,ch}_{k,k+q,k'-k}+\frac{1}{2}\Delta^{\rm ph,sp}_{k,k+q,k'-k}\right)\\&=-\frac{2r-1}{2}\Delta^{\rm ph,ch}_{k,k+q,k'-k}-\frac{2r+1}{2}\Delta^{\rm ph,sp}_{k,k+q,k'-k}.\end{aligned} \tag{S13}$$

Inserting Eq. (S11c) into the expression inside the square bracket in the third line, we obtain

$$\begin{aligned}r\Delta^{\rm pp,ch}_{kk',k+k'+q}+(r-1)\Delta^{\rm pp,sp}_{kk',k+k'+q}&=\frac{r}{2}\Delta^{\rm pp,si}_{kk',k+k'+q}-\frac{r-1}{2}\Delta^{\rm pp,si}_{kk',k+k'+q}\\&=\frac{1}{2}\Delta^{\rm pp,si}_{kk',k+k'+q}.\end{aligned} \tag{S14}$$

By setting $U^{\rm ch}$ to $U$ and $U^{\rm sp}$ to $-U$, we can simplify the expression inside the square bracket in the last line as

$$rU^{\rm ch}+(r-1)U^{\rm sp}=U. \tag{S15}$$

After these simplifications, we get

$$\begin{aligned}
\Sigma_k - \Sigma^H =& - U \sum_{k'q} G_{k+q} G_{k'} G_{k'+q} \left[ r \Delta^{\text{ph,ch}}_{kk'q} + (r-1) \Delta^{\text{ph,sp}}_{kk'q} \right] \\
&+ U \sum_{k'q} G_{k+q} G_{k'} G_{k'+q} \left[ \frac{2r-1}{2} \Delta^{\text{ph,ch}}_{k,k+q,k'-k} + \frac{2r+1}{2} \Delta^{\text{ph,sp}}_{k,k+q,k'-k} \right] \\
&- \frac{U}{2} \sum_{k'q} G_{k+q} G_{k'} G_{k'+q} \Delta^{\text{pp,si}}_{kk',k+k'+q} \\
&- U \sum_{k'q} G_{k+q} G_{k'} G_{k'+q} \left[ r \Lambda^{\text{Uirr,ch}}_{kk'q} + (r-1) \Lambda^{\text{Uirr,sp}}_{kk'q} \right] \\
&+ 2U^2 \sum_{k'q} G_{k+q} G_{k'} G_{k'+q}.
\end{aligned} \tag{S16}$$

We can further rewrite the second line with $\tilde{k}' = k+q$ and $\tilde{q} = k'-k$:

$$\begin{aligned}
& U \sum_{k'q} G_{k+q} G_{k'} G_{k'+q} \left[ \frac{2r-1}{2} \Delta^{\text{ph,ch}}_{k,k+q,k'-k} + \frac{2r+1}{2} \Delta^{\text{ph,sp}}_{k,k+q,k'-k} \right] \\
&= U \sum_{\tilde{k}'\tilde{q}} G_{\tilde{k}'} G_{k+\tilde{q}} G_{\tilde{k}'+\tilde{q}} \left[ \frac{2r-1}{2} \Delta^{\text{ph,ch}}_{k\tilde{k}'\tilde{q}} + \frac{2r+1}{2} \Delta^{\text{ph,sp}}_{k\tilde{k}'\tilde{q}} \right] \\
&= U \sum_{k'q} G_{k+q} G_{k'} G_{k'+q} \left[ \frac{2r-1}{2} \Delta^{\text{ph,ch}}_{kk'q} + \frac{2r+1}{2} \Delta^{\text{ph,sp}}_{kk'q} \right],
\end{aligned} \tag{S17}$$

where we rename $\tilde{k}'$ and $\tilde{q}$ as $k'$ and $q$, respectively, at the end. Similarly, for the third line, let $\tilde{q} = k+k'+q$, we obtain

$$\begin{aligned}
& - \frac{U}{2} \sum_{k'q} G_{k+q} G_{k'} G_{k'+q} \Delta^{\text{pp,si}}_{kk',k+k'+q} \\
&= - \frac{U}{2} \sum_{k'\tilde{q}} G_{\tilde{q}-k'} G_{k'} G_{\tilde{q}-k} \Delta^{\text{pp,si}}_{kk'\tilde{q}} \\
&= - \frac{U}{2} \sum_{k'q} G_{q-k'} G_{k'} G_{q-k} \Delta^{\text{pp,si}}_{kk'q},
\end{aligned} \tag{S18}$$

where we rename $\tilde{q}$ as $q$ at the end.

Now we are ready to see

$$\begin{aligned}
\Sigma_k - \Sigma^H =& - \frac{U}{2} \sum_{k'q} G_{k+q} G_{k'} G_{k'+q} \Delta^{\text{ph,ch}}_{kk'q} \\
&+ \frac{3U}{2} \sum_{k'q} G_{k+q} G_{k'} G_{k'+q} \Delta^{\text{ph,sp}}_{kk'q} \\
&- \frac{U}{2} \sum_{k'q} G_{q-k'} G_{k'} G_{q-k} \Delta^{\text{pp,si}}_{kk'q} \\
&- U \sum_{k'q} G_{k+q} G_{k'} G_{k'+q} \left[ r \Lambda^{\text{Uirr,ch}}_{kk'q} + (r-1) \Lambda^{\text{Uirr,sp}}_{kk'q} \right] \\
&+ 2U^2 \sum_{k'q} G_{k+q} G_{k'} G_{k'+q}.
\end{aligned} \tag{S19}$$

Next, we use Eqs. (2), (3), and (4) of Ref. [1]:

$$\begin{aligned}
&\Delta^{\mathrm{ph,ch/sp}}_{kk'q} = \gamma^{\mathrm{ch/sp}}_{kq} W^{\mathrm{ch/sp}}_{q} \gamma^{\mathrm{ch/sp}}_{k'q}, && \Delta^{\mathrm{pp,si}}_{kk'q} = \gamma^{\mathrm{si}}_{kq} W^{\mathrm{si}}_{q} \gamma^{\mathrm{si}}_{k'q};\\
&\sum_{k'} \gamma^{\mathrm{ch/sp}}_{k'q} G_{k'} G_{k'+q} = \Pi^{\mathrm{ch/sp}}_{q}, && \sum_{k'} \gamma^{\mathrm{si}}_{k'q} G_{k'} G_{q-k'} = \Pi^{\mathrm{si}}_{q};\\
&W^{\mathrm{ch/sp}}_{q} \Pi^{\mathrm{ch/sp}}_{q} U^{\mathrm{ch/sp}}_{q} = W^{\mathrm{ch/sp}}_{q} - U^{\mathrm{ch/sp}}, && W^{\mathrm{si}}_{q} \Pi^{\mathrm{si}}_{q} \frac{1}{2} U^{\mathrm{si}} = W^{\mathrm{si}}_{q} - U^{\mathrm{si}};
\end{aligned} \tag{S20}$$

where $\Pi$ denotes the polarization, and obtain

$$\begin{aligned}
\Sigma_k - \Sigma^H = &-\frac{1}{2} \sum_{k'q} G_{k+q} \gamma^{\mathrm{ch}}_{kq} (W^{\mathrm{ch}}_{q} - U^{\mathrm{ch}})\\
&-\frac{3}{2} \sum_{k'q} G_{k+q} \gamma^{\mathrm{sp}}_{kq} (W^{\mathrm{sp}}_{q} - U^{\mathrm{sp}})\\
&-\frac{1}{2} \sum_{k'q} G_{q-k} \gamma^{\mathrm{si}}_{kq} (W^{\mathrm{si}}_{q} - U^{\mathrm{si}})\\
&-U \sum_{k'q} G_{k+q} G_{k'} G_{k'+q} \left[ r \Lambda^{\mathrm{Uirr,ch}}_{kk'q} + (r-1) \Lambda^{\mathrm{Uirr,sp}}_{kk'q} \right]\\
&+2U^2 \sum_{k'q} G_{k+q} G_{k'} G_{k'+q}.
\end{aligned} \tag{S21}$$

We consider the weak-coupling (second order in $U$) limit for the first three terms

$$\begin{aligned}
&-\frac{1}{2} \sum_{q} G_{k+q} \gamma^{\mathrm{ch}}_{kq} (W^{\mathrm{ch}}_{q} - U^{\mathrm{ch}}) \approx -\frac{U^2}{2} \sum_{k'q} G_{k+q} G_{k'} G_{k'+q},\\
&-\frac{3}{2} \sum_{q} G_{k+q} \gamma^{\mathrm{sp}}_{kq} (W^{\mathrm{sp}}_{q} - U^{\mathrm{sp}}) \approx -\frac{3U^2}{2} \sum_{k'q} G_{k+q} G_{k'} G_{k'+q},\\
&-\frac{1}{2} \sum_{q} G_{q-k} \gamma^{\mathrm{si}}_{kq} (W^{\mathrm{si}}_{q} - U^{\mathrm{si}}) \approx -U^2 \sum_{k'q} G_{q-k} G_{k'} G_{q-k'} = -\frac{2U^2}{2} \sum_{k'q} G_{k+q} G_{k'} G_{k'+q}.
\end{aligned}$$

We can rewrite the results with the weak-coupling limit subtracted from corresponding terms

$$\begin{aligned}
\Sigma_k - \Sigma^H = &-\frac{1}{2} \sum_{k'q} G_{k+q} \gamma^{\mathrm{ch}}_{kq} (W^{\mathrm{ch}}_{q} - U^{\mathrm{ch}}) + \frac{U^2}{2} \sum_{k'q} G_{k+q} G_{k'} G_{k'+q}\\
&-\frac{3}{2} \sum_{k'q} G_{k+q} \gamma^{\mathrm{sp}}_{kq} (W^{\mathrm{sp}}_{q} - U^{\mathrm{sp}}) + \frac{3U^2}{2} \sum_{k'q} G_{k+q} G_{k'} G_{k'+q}\\
&-\frac{1}{2} \sum_{k'q} G_{q-k} \gamma^{\mathrm{si}}_{kq} (W^{\mathrm{si}}_{q} - U^{\mathrm{si}}) + \frac{2U^2}{2} \sum_{k'q} G_{k+q} G_{k'} G_{k'+q}\\
&-U \sum_{k'q} G_{k+q} G_{k'} G_{k'+q} \left[ r \Lambda^{\mathrm{Uirr,ch}}_{kk'q} + (r-1) \Lambda^{\mathrm{Uirr,sp}}_{kk'q} \right]\\
&-U^2 \sum_{k'q} G_{k+q} G_{k'} G_{k'+q}.
\end{aligned} \tag{S22}$$

Finally, we apply Eq. (S6) and as the result we obtain the unambiguous self-energy decomposition

$$\Sigma_k - \Sigma^H = \Sigma^{\mathrm{mb}}_{k} + \Sigma^{\mathrm{2nd}}_{k} + \Sigma^{\mathrm{ch}}_{k} + \Sigma^{\mathrm{sp}}_{k} + \Sigma^{\mathrm{si}}_{k}, \tag{S23}$$

with $\Sigma^{\rm 2nd}, \Sigma^{\rm ch}, \Sigma^{\rm sp}, \Sigma^{\rm si}$ defined in the main text

$$\Sigma_k^{\rm 2nd} = -U^2 \sum_{k'q} G_{k+q} G_{k'} G_{k'+q}, \tag{S24a}$$

$$\Sigma_k^{\rm ch} = -\frac{U^2}{2} \sum_q G_{k+q} \gamma_{kq}^{\rm ch} \chi_q^{\rm ch} - \frac{1}{2} \Sigma_k^{\rm 2nd}, \tag{S24b}$$

$$\Sigma_k^{\rm sp} = -\frac{3U^2}{2} \sum_q G_{k+q} \gamma_{kq}^{\rm sp} \chi_q^{\rm sp} - \frac{3}{2} \Sigma_k^{\rm 2nd}, \tag{S24c}$$

$$\Sigma_k^{\rm si} = -U^2 \sum_q G_{q-k} \gamma_{kq}^{\rm si} \chi_q^{\rm si} - \Sigma_k^{\rm 2nd}, \tag{S24d}$$

and

$$\Sigma_k^{\rm mb} = -\,U \sum_{k'q} G_{k+q} G_{k'} G_{k'+q} \left[ r \Lambda_{kk'q}^{\rm Uirr,ch} + (r-1) \Lambda_{kk'q}^{\rm Uirr,sp} \right]. \tag{S25}$$

All terms in Eq. (S23) are unequivocally defined independent of $r$, except for $\Sigma^{\rm mb}$ which has a $r$-dependent decomposition on the right-hand side. This term is, however, anyhow, a multi-boson contribution beyond a mere contribution of a single bosonic mode.

As a side note, we find the term $-U^2 \sum_q G_{q-k} \gamma_{kq}^{\rm si} \chi_q^{\rm si}$ in the singlet contribution (Eq. S24d) is hard to converge at low frequencies with the finite frequency box used in our calculation. Therefore, we use the expression before the momentum-frequency shift [see Eq. (S18)], $-\frac{U}{2} \sum_{k'q} G_{k+q} G_{k'} G_{k'+q} \Delta^{\rm pp,si}_{kk',k+k'+q}$, for most of our calculations. This expression converges better at low frequencies but worse at high frequencies. The only place where we directly use Eq. (S24d) is in Fig. 2, where we discuss the asymptotic behavior of different terms in the decomposition and need a better convergence at high frequencies. A direct measurement of Hedin vertices in quantum Monte Carlo would improve the convergence issue, but it was not implemented for this study.

## III. ADDITIONAL RESULTS

### A. Dynamical mean-field theory

For comparison with DCA we apply the fluctuation decomposition presented in the main text to DMFT calculations for the Hubbard model on the half-filled square lattice ($T = 0.2t$, $t' = 0$). In Fig. 1 we observe the various terms in Eq. (S23) for different coupling strengths $U/t = 2$, 6, and 10. Similar to DCA, $\mathrm{Im}\Sigma^{\rm mb}$ is large and positive for large $U$, canceling (similarly as in DCA) about half of the (local) DMFT spin fluctuations. While similar in magnitude as in DCA, the different DMFT self-energy contributions, as a matter of course, do not have a momentum differentiation. Thus, for $U = 6t$ we still see a metallic negative slope of the DMFT self-energy, whereas for $U = 10t$ we see an insulating-like positive slope. Note $U = 10t$ is close to the lower critical $U$ of the first-order Mott transition. Given the temperature $T = 0.2t$ we are, however, above the critical point of the first-order phase transition, i.e., in the non-critical crossover regime between metal and insulator. The DMFT self-energy also has a large contribution from the singlet channel (si) at weak and intermediate $U$. Such a large particle-particle channel contribution has been observed in the vertex [8], but to our best knowledge not in the self-energy before.

Fig. 2 shows the high-frequency asymptote of the self-energy for Matsubara frequencies $\nu$ at $U = 2t$ in DMFT. This highlights that $\Sigma^{\rm ch}, \Sigma^{\rm sp}, \Sigma^{\rm si}$ have finite contributions $\propto \frac{1}{\nu}$, however, they cancel out exactly and $\Sigma^{\rm 2nd}$ alone recovers the generic asymptote $U^2 \frac{\langle \hat{n} \rangle}{2} (1 - \frac{\langle \hat{n} \rangle}{2})/\nu$. Also, note that the multi-boson contribution $\Sigma^{\rm mb}$ decays faster than $1/\nu$. As discussed in the previous section, here we use Eq. (S24d) to calculate $\Sigma^{\rm si}$ to achieve better convergence for high frequencies. To also achieve good convergence at low frequencies, we evaluate the Hedin vertices in Eq. (S24) and Eq. (S25) over a wide frequency window. The number of bosonic and fermionic Matsubara frequencies used for the Hedin vertices here are 201 and 200 respectively.

Fig. 3 shows the Hedin vertex $\gamma^{\rm sp}(\nu, \omega = 0)$ as a function of $\nu$ for various $U$. For small frequencies, the vertex is suppressed for small $U$ and enhanced for large $U$, in particular in the Mott insulating regime at $U = 10t$ [9].

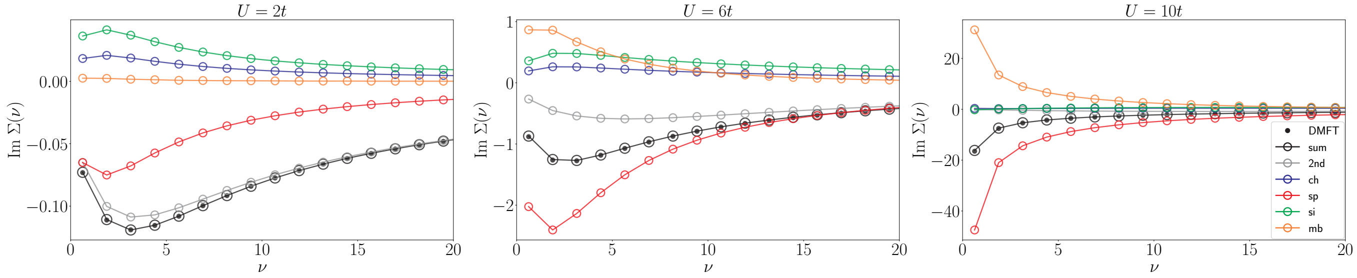


FIG. 1. Decomposition according to Eq. (S23) of the DMFT self-energy for various interactions $U$ from weak to strong coupling (half-filled square lattice, $T = 0.2t$).

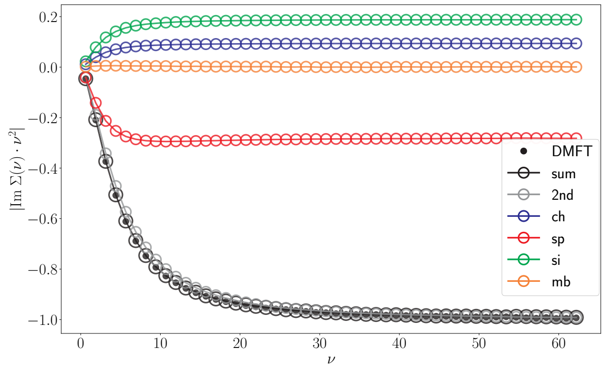


FIG. 2. High-frequency asymptote of the DMFT self-energy for $U = 2t$, obtained by multiplying Fig. 1 (left panel) with $\nu$ and displaying a larger frequency range.

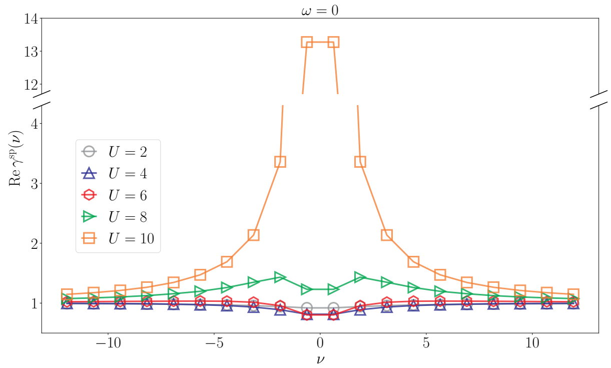


FIG. 3. Real part of the Matsubara Hedin spin-fermion vertex $\gamma^{\mathrm{sp}}(\nu, \omega = 0)$ within DMFT for various $U$ (half-filled square lattice, $T = 0.2t$). The imaginary part vanishes due to particle-hole symmetry.

### B. Dynamical cluster approximation

Fig. 4 shows the fluctuation decomposition of the real and imaginary part of the self-energy. The top panels correspond to the pseudogap regime ($\langle \hat{n} \rangle = 0.95$) discussed in the main text, bottom panels to the metallic, overdoped regime ($\langle \hat{n} \rangle = 0.9$). In the overdoped case shown here, both nodal and antinodal momenta exhibit a metallic behavior of the self-energy $\Sigma$ (negative slope of its imaginary part at low Matsubara frequencies). The spin fluctuation contribution $\Sigma^{\mathrm{sp}}$ also displays metallic behavior at both momenta in this overdoped regime. The magnitude of $\Sigma^{\mathrm{mb}}$ is comparable inside and outside the pseudogap regime. However, its slope at small Matsubara frequencies changes sign, similar (but opposite) to $\Sigma^{\mathrm{sp}}$.

In Figs. 5 and 6 we diagnose the **q**- and $\omega$-dependence of our fluctuation decomposition in the pseudogap regime and for overdoping, respectively. That is, we study the **q**- and $\omega$-dependent contribution of all the terms in Eq. (S23).

For the multi-boson term $\Sigma^{\text{mb}}$ the Fierz ambiguity remains and this analysis is akin to the fluctuation diagnostics [7]. Here, we thus show different decoupling parameters $r = 0, 1, \frac{1}{4}$, and $\frac{1}{2}$. We remind that the first three of these choices correspond to the spin, charge, or singlet picture, respectively, cf. Sec. II and Ref. [7]. The last option $r = \frac{1}{2}$ simply corresponds to an even splitting between the charge and spin channels.

The only contribution with a clear-cut peak of its momentum distribution is the single-boson spin channel (sp) which has its major contribution from spin fluctuations around $\mathbf{q} = (\pi, \pi)$. It also peaks at Matsubara frequency $\omega = 0$, indicating thermal fluctuations. The charge and singlet single-boson contributions have neither a pronounced momentum nor frequency dependence and are also smaller, signaling the absence of a relevant charge or singlet boson.

More complicated, because of the lack of an unambiguous decomposition, is the multi-boson contribution, which is also sizable and hence important. Here, for *all* decoupling parameters $r$, we do not find a peak in the $\mathbf{q}$-resolved $\Sigma^{\text{mb}}$. Hence, the multi-boson contribution is not simply a variant of the $\mathbf{q} = (\pi, \pi)$ spin fluctuations. In the analysis of its $\omega$-dependence we see a sizable $\omega = 0$ contribution, but it is truly dominant only for the singlet channel ($r = 1/4$; last row of circles in Figs. 5 and 6). Interestingly, the emphasis of $\Sigma^{\text{mb}}$ on $\omega = 0$ is less strong in the pseudogap regime than for overdoping.

Finally, Fig. 7 shows the fermion-boson (Hedin) vertex $\gamma^{\text{sp}}(\mathbf{k}, \nu, \mathbf{q}, \omega)$ for $\mathbf{q} = (\pi, \pi), \omega = 0$, which couples static antiferromagnetic spin fluctuations to fermions with momentum $\mathbf{k}$ and Matsubara frequency $\nu$. We show the contributions for $\mathbf{k} = (\pi, 0)$ (left) and $(\frac{\pi}{2}, \frac{\pi}{2})$ (right). Consistent with Ref. [10] the vertex exhibits a sizable negative (positive) imaginary part for positive (negative) Matsubaras, however, we observe an enhancement of its real part for antinodal fermions in the pseudogap regime (circles, top left), reminiscent of the DMFT Mott insulator, cf. Fig. 3. This feature is hard to capture with the method employed in Ref. [10], which corresponds to a perturbation theory around a metallic DMFT solution. At the node (squares) the vertex is suppressed, similar to a metallic DMFT solution (cf. Fig. 3) and Ref. [10]. The impact of the imaginary part on the momentum structure of the pseudogap differs qualitatively from the real part [10], however, it can not be investigated here due to the coarse momentum resolution of the cluster.

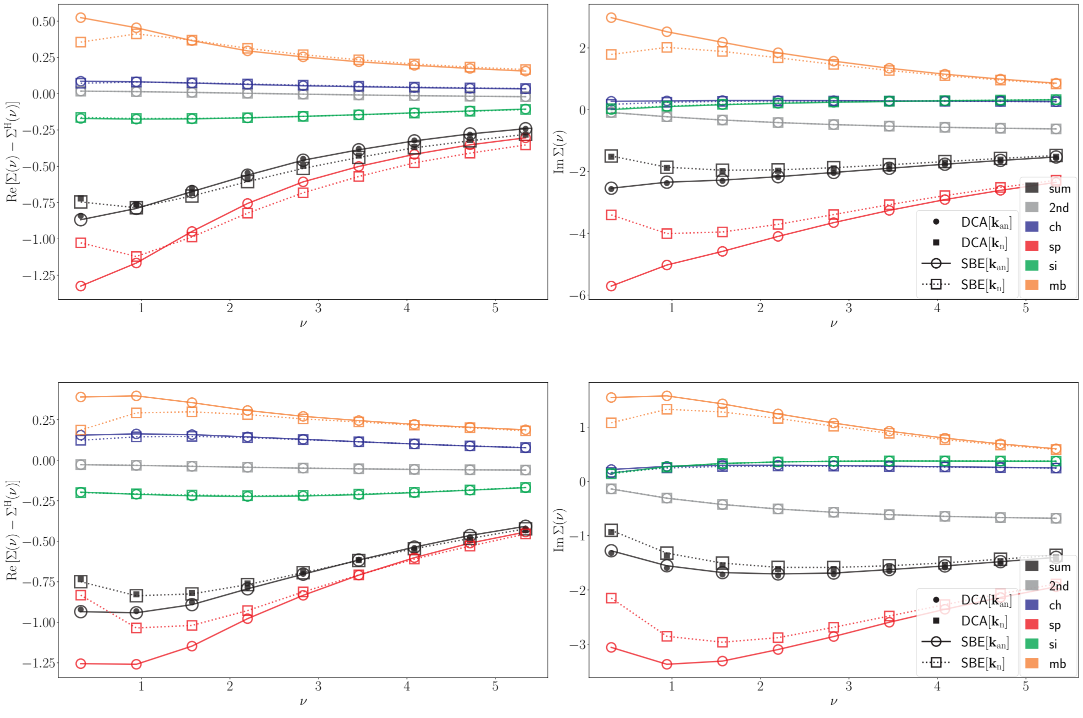


FIG. 4. Decomposition of the real (left) and imaginary part (right) of the 8-site DCA self-energy in the pseudogap regime (top, $\langle \hat{n} \rangle = 0.95$) and for overdoping (bottom, $\langle \hat{n} \rangle = 0.9$). Parameters: $U = 7t, t' = -0.15t, T/t = 0.1$; colors and labels as in the main text.

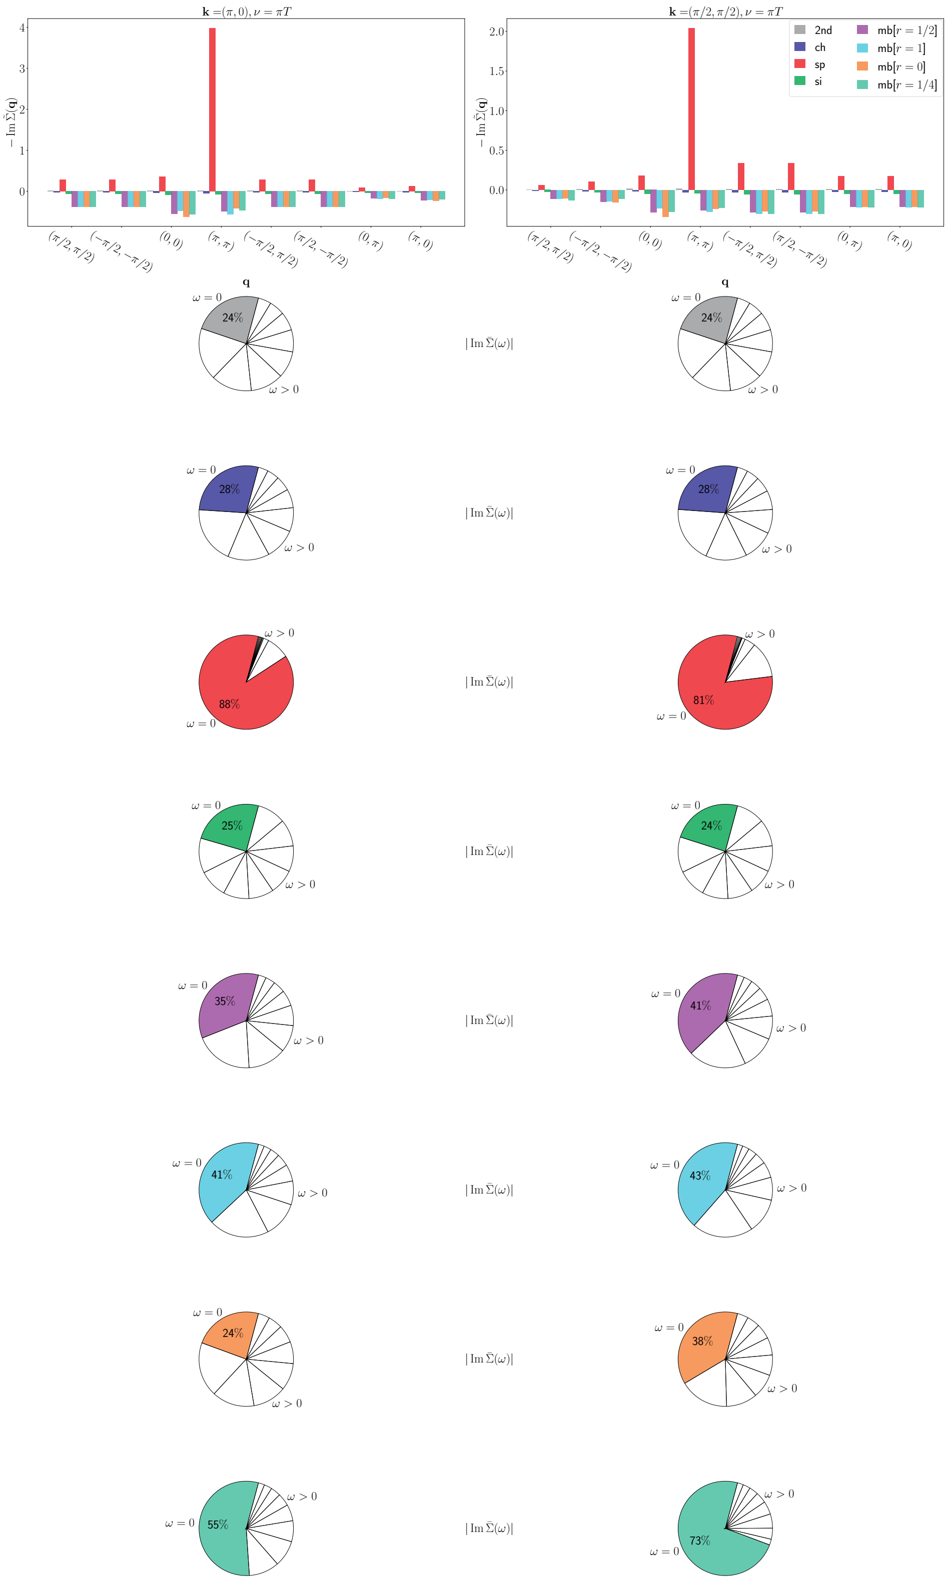


FIG. 5. Complete fluctuation decomposition in the pseudogap regime ($\langle \hat{n} \rangle = 0.95$), showing the unambiguous contributions to Eq. (S23) ($\Sigma^{\mathrm{2nd}}, \Sigma^{\mathrm{ch}}, \Sigma^{\mathrm{sp}}, \Sigma^{\mathrm{si}}$) and $\Sigma^{\mathrm{mb}}$ using four different choices of the decoupling parameter $r$ for the latter. Bar charts: **q**-resolved fluctuation decomposition of the antinodal (left) and nodal (right) self-energy ($\nu = \pi T$). Pie charts: $\omega$-resolved fluctuation decomposition. Parameters as in Fig. 4.

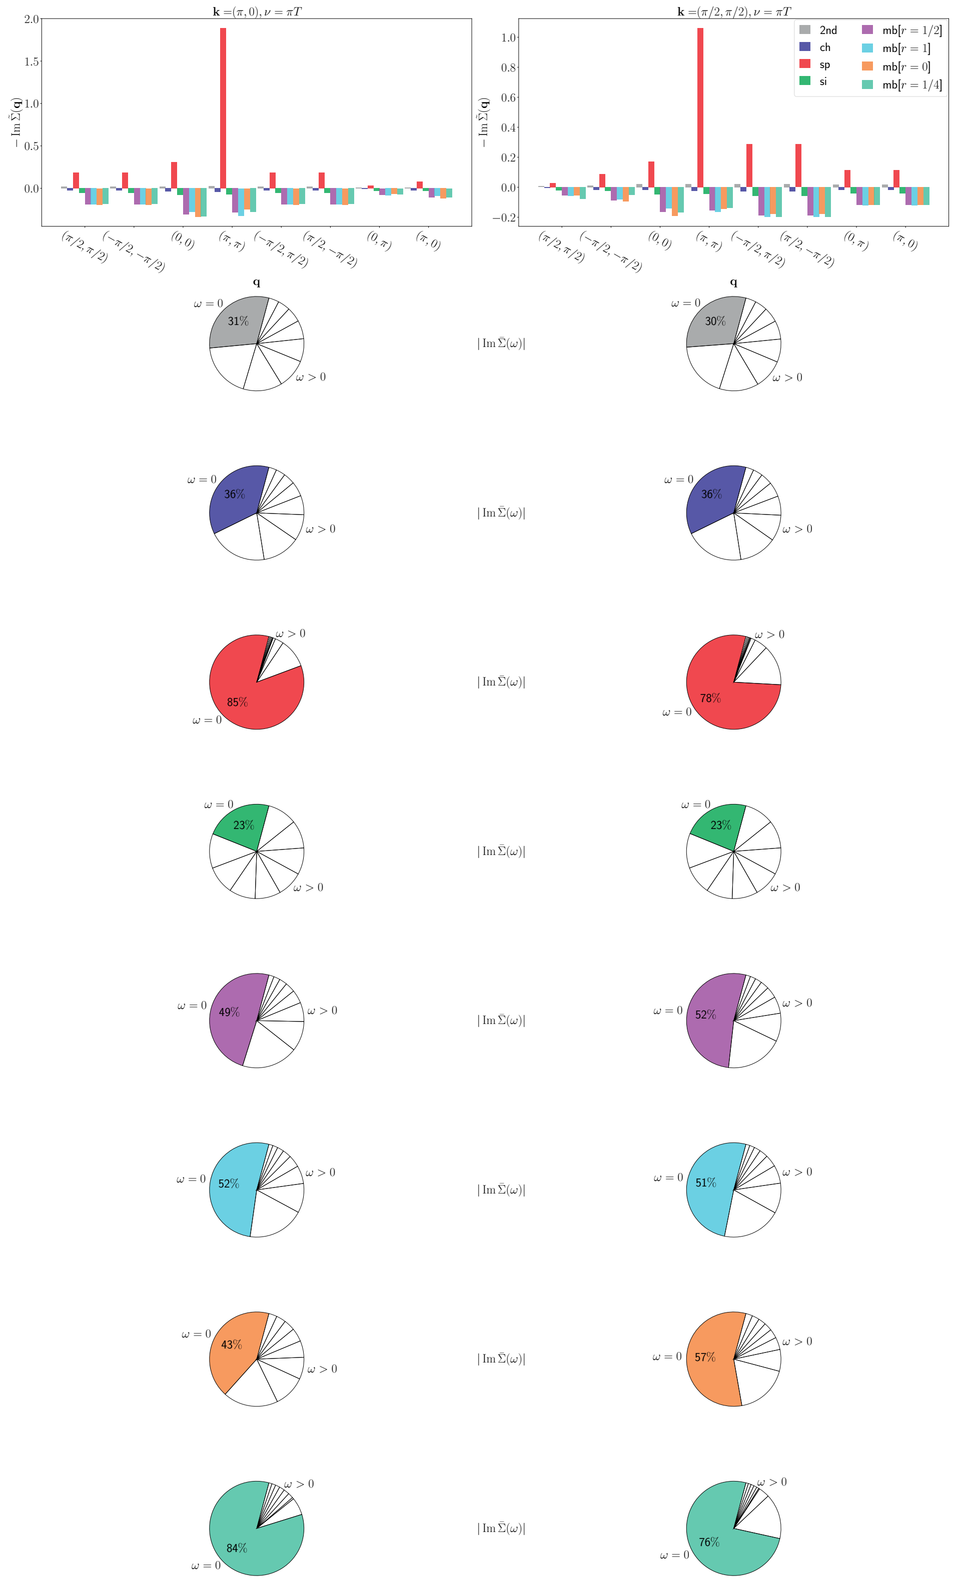


FIG. 6. Complete fluctuation decomposition as in Fig. 5 but now for overdoping ($\langle \hat{n} \rangle = 0.9$).

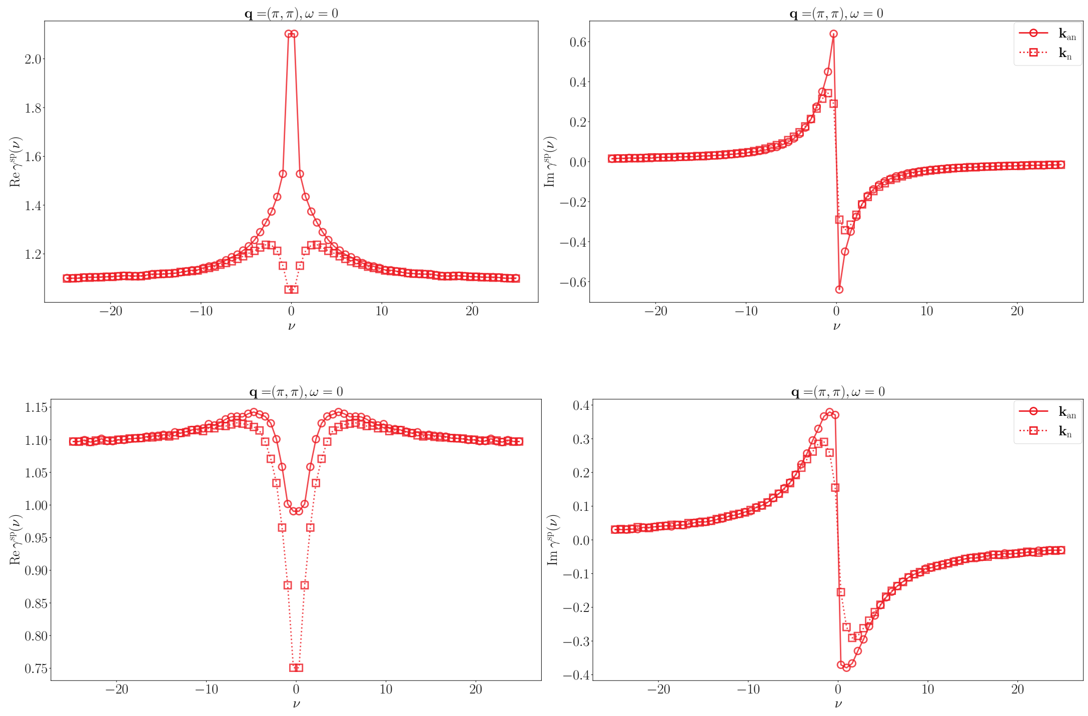


FIG. 7. Real (left) and imaginary (right) part of the Hedin vertex as a function of fermionic Matsubara frequency $\nu$ in the pseudogap regime (top, $\langle\hat{n}\rangle = 0.95$) and for overdoping (bottom, $\langle\hat{n}\rangle = 0.9$). Parameters as in Fig. 4.


[1] F. Krien, A. Kauch, and K. Held, Phys. Rev. Research **3**, 013149 (2021).
[2] A. N. Rubtsov, V. V. Savkin, and A. I. Lichtenstein, Phys. Rev. B **72**, 035122 (2005).
[3] P. Werner, A. Comanac, L. de' Medici, M. Troyer, and A. J. Millis, Phys. Rev. Lett. **97**, 076405 (2006).
[4] E. Gull, P. Werner, O. Parcollet, and M. Troyer, Europhysics Letters **82**, 57003 (2008).
[5] E. Gull, A. J. Millis, A. I. Lichtenstein, A. N. Rubtsov, M. Troyer, and P. Werner, Rev. Mod. Phys. **83**, 349 (2011).
[6] F. Krien, A. Valli, and M. Capone, Phys. Rev. B **100**, 155149 (2019).
[7] O. Gunnarsson, T. Schäfer, J. P. F. LeBlanc, E. Gull, J. Merino, G. Sangiovanni, G. Rohringer, and A. Toschi, Phys. Rev. Lett. **114**, 236402 (2015).
[8] M. Kitatani, T. Schäfer, H. Aoki, and K. Held, Phys. Rev. B **99**, 041115 (2019).
[9] V. Harkov, A. I. Lichtenstein, and F. Krien, Phys. Rev. B **104**, 125141 (2021).
[10] F. Krien, P. Worm, P. Chalupa-Gantner, A. Toschi, and K. Held, Communications Physics **5** (2022), 10.1038/s42005-022-01117-5.
